# Supplementary material for: Large-scale chaos and fluctuations in active nematics
Source: arXiv:1312.1076 source file (2013-12-04)
Supplement: Supplementary file 1 [file supplement.pdf]

## I. TRANSVERSE INSTABILITY OF THE BAND

To examine stability of the band solution with respect to transversal undulations, we rewrite Eqs. (1), (2) (main text) for real and imaginary parts, $f_1 = U + iV$, yielding

$$\partial_t \rho = \frac{1}{2}\Delta\rho + \frac{1}{2}\left((\partial_x^2 - \partial_y^2)U + 2\partial_x\partial_y V\right) \tag{1}$$

$$\partial_t U = (\mu_0 - \xi(U^2+V^2)U + \mu'\rho U + \frac{1}{4}(\partial_x^2 - \partial_y^2)\rho + \frac{1}{2}\Delta U \tag{2}$$

$$\partial_t V = (\mu_0 - \xi(U^2+V^2)V + \mu'\rho V + \frac{1}{2}\partial_x\partial_y\rho + \frac{1}{2}\Delta V \tag{3}$$

Here we define $\mu_0 = -\rho_t\mu'$. Band solution (Eq. (4), main text) assumes the form $U = U_0(y), V = 0, \rho = U_0(y) + \rho_{\text{gas}} \equiv R_0(y)$. We seek perturbative solution to Eqs. (1)-(3) in the form $U = U_0 + u(y)\exp[ikx+\lambda t], V = v(y)\exp[ikx+\lambda t], \rho = R_0(y) + r(y)\exp[ikx+\lambda t]$, which results in the following linearized system

$$\lambda r = \frac{1}{2}(\partial_y^2 - k^2)r - \frac{1}{2}(k^2 + \partial_y^2)u + ik\partial_y v \tag{4}$$

$$\lambda u = (\mu_0 - 3\xi U_0^2)u + \mu' R_0 u + \mu' U_0 r - \frac{1}{4}(k^2 + \partial_y^2)r + \frac{1}{2}(\partial_y^2 - k^2)u \tag{5}$$

$$\lambda v = (\mu_0 - \xi U_0^2)v + \mu' R_0 v + \frac{1}{2}ik\partial_y r + \frac{1}{2}(\partial_y^2 - k^2)v \tag{6}$$

Due to translational symmetry, for $k = 0$ there exists a stationary solution ($\lambda = 0$) to the linearized system Eqs. (4)-(6) in the form $v = 0, u = \partial_y U_0(y), r = \partial_y U_0(y)$. Therefore, for $k \to 0$ we can seek perturbative solution as follows (we define $\lambda = \lambda_1 k^2$)

$$\begin{pmatrix} r(y) \\ u(y) \\ v(y) \end{pmatrix} = \begin{pmatrix} \partial_y U_0(y) \\ \partial_y U_0(y) \\ 0 \end{pmatrix} + \begin{pmatrix} k^2 r_1(y) \\ k^2 u_1(y) \\ ikv_1(y) \end{pmatrix} \tag{7}$$

As we will show later, this specific form of the expansion with respect to small parameter $k$ yields nontrivial result for the eigenvalue $\lambda$. After substitution of (7) into Eqs. (4)-(6) we obtain in the first non-trivial order

$$\lambda_1\partial_y U_0 + \partial_y U_0 = \frac{1}{2}\partial_y^2 r_1 - \frac{1}{2}\partial_y^2 u_1 - \partial_y v_1 \tag{8}$$

$$\lambda_1\partial_y U_0 + \frac{3}{4}\partial_y U_0 = (\mu_0 - 3\xi U_0^2)u_1 + \mu' R_0 u_1 + \mu' U_0 r_1 - \frac{1}{4}\partial_y^2 r_1 + \frac{1}{2}\partial_y^2 u_1 \tag{9}$$

$$-\frac{1}{2}\partial_y^2 U_0 = (\mu_0 - \xi U_0^2)v_1 + \mu' R_0 v_1 + \frac{1}{2}\partial_y^2 v_1 \tag{10}$$

One can check that exact solution to Eq. (10) is $v_1 = -2U_0$. So, the remaining equations can be written as

$$(\lambda_1 - 1)\partial_y U_0 = \frac{1}{2}\partial_y^2 r_1 - \frac{1}{2}\partial_y^2 u_1 \tag{11}$$

$$\left(\lambda_1 + \frac{3}{4}\right)\partial_y U_0 = (\mu_0 - 3\xi U_0^2)u_1 + \mu' R_0 u_1 + \mu' U_0 r_1 - \frac{1}{4}\partial_y^2 r_1 + \frac{1}{2}\partial_y^2 u_1 \tag{12}$$

It is convenient to introduce a new variable $w = r_1 - u_1$. Then Eqs. (11),(12) assume the form

$$(\lambda_1 - 1)\partial_y U_0 = \frac{1}{2}\partial_y^2 w \tag{13}$$

$$\left(\lambda_1 + \frac{3}{4}\right)\partial_y U_0 = (\mu_0 - 3\xi U_0^2)u_1 + \mu' R_0 u_1 + \mu' U_0(w + u_1) - \frac{1}{4}\partial_y^2 w + \frac{1}{4}\partial_y^2 u_1 \tag{14}$$

Substituting $\partial_y^2 w$ from Eq. (13) into Eq. (14) results in

$$(\lambda_1 - 1)\partial_y U_0 = \frac{1}{2}\partial_y^2 w \tag{15}$$

$$\left(\frac{3}{2}\lambda_1 + \frac{1}{4}\right)\partial_y U_0 = (\mu_0 - 3\xi U_0^2)u_1 + \mu' R_0 u_1 + \mu' U_0(w + u_1) + \frac{1}{4}\partial_y^2 u_1 \tag{16}$$

Integration of Eq. (15) gives rise to an explicit expression for $w$:

$$w = 2(\lambda_1 - 1)\int dy\, U_0(y) \tag{17}$$

Using Eq. (17), we derive from Eq. (16) an inhomogeneous second-order differential equation for the function $u_1$:

$$\left(\frac{3}{2}\lambda_1 + \frac{1}{4}\right)\partial_y U_0 - 2\mu' U_0(\lambda_1 - 1)\int dy\, U_0(y) = (\mu_0 - 3\xi U_0^2)u_1 + \mu' R_0 u_1 + \mu' U_0 u_1 + \frac{1}{4}\partial_y^2 u_1 \tag{18}$$

It is convenient to rewrite formally the above equation as $B(y) = \mathcal{L}u_1(y)$, where $B(y)$ is the l.h.s. of Eq. (18) and $\mathcal{L}$ is the differential operator defined as

$$\mathcal{L} = (\mu_0 - 3\xi U_0^2) + \mu' R_0 + \mu' U_0 + \frac{1}{4}\partial_y^2 \tag{19}$$

The operator $\mathcal{L}$ is self-adjoint with respect to the scalar product of functions defined as $\langle \psi_1, \psi_2\rangle = \int_{-\infty}^{\infty} dy\, \psi_1(y)\psi_2(y)$, meaning that for any functions $\psi_1$ and $\psi_2$, $\langle \mathcal{L}\psi_1, \psi_2\rangle = \langle \psi_1, \mathcal{L}\psi_2\rangle$. It is easy to check that $\mathcal{L}$ possesses a localized zero eigenmode $\psi_0(y) = \partial_y U_0(y)$. Therefore, taking the scalar product of Eq. (18) by $\psi_0(y)$, one finds

$$\langle \psi_0, B\rangle = \langle \psi_0, \mathcal{L}u_1\rangle \tag{20}$$

Thanks to the self-adjoint property, one has $\langle \psi_0, \mathcal{L}u_1\rangle = \langle \mathcal{L}\psi_0, u_1\rangle = 0$, eventually yielding $\langle \psi_0, B\rangle = 0$, a condition called solvability condition. In more explicit terms, this condition reads

$$\int_{-\infty}^{\infty} dy\, \partial_y U_0 \left(\left(\frac{3}{2}\lambda_1 + \frac{1}{4}\right)\partial_y U_0 - 2\mu' U_0(\lambda_1 - 1)\int dy\, U_0(y)\right) = 0 \tag{21}$$

It can be simplified by integrating by parts the second term in the above integral, leading to

$$\left(\frac{3}{2}\lambda_1 + \frac{1}{4}\right)\int_{-\infty}^{\infty} dy\, (\partial_y U_0)^2 + (\lambda_1 - 1)\mu' \int_{-\infty}^{\infty} dy\, U_0(y)^3 = 0 \tag{22}$$

The solvability condition (22) can be written as $\lambda_1 g + d = 0$. One immediately sees that

$$g = \frac{3}{2}\int_{-\infty}^{\infty} dy\, (\partial_y U_0)^2 + \mu' \int_{-\infty}^{\infty} dy\, U_0(y)^3 > 0 \tag{23}$$

Therefore, the band solution is unstable ($\lambda_1 > 0$) if the following condition is fulfilled

$$d = \frac{1}{4}\int_{-\infty}^{\infty} dy(\partial_y U_0)^2 - \mu' \int_{-\infty}^{\infty} dy\, U_0(y)^3 < 0 \tag{24}$$

Now we evaluate Eq. (23) by substituting the band solution (Eq. (4), main text) in the form

$$U_0(y) = \frac{c}{1 + a\cosh(by)} \tag{25}$$

where positive parameters $a, b, c$ are of the form

$$c = 3(\rho_t - \rho_{\mathrm{gas}}), \quad a = \sqrt{1 - 9\xi(\rho_t - \rho_{\mathrm{gas}})/2\mu'}, \quad b = 2\sqrt{\mu'(\rho_t - \rho_{\mathrm{gas}})} \tag{26}$$

Evaluation of Eq. (24) using the band solution Eq. (24) gives rise to a relatively simple analytical expression for $d$, using the relation $\mu' c = 3b^2/4$,

$$d = \frac{1}{4}c^2 b f(a) \tag{27}$$

where the function $f(a)$ is given by

$$f(a) = \int_{-\infty}^{\infty} dx\, \left(\phi_a'(x)^2 - 3\phi_a(x)^3\right), \qquad \phi_a(x) = \frac{1}{1 + a\cosh x} \tag{28}$$

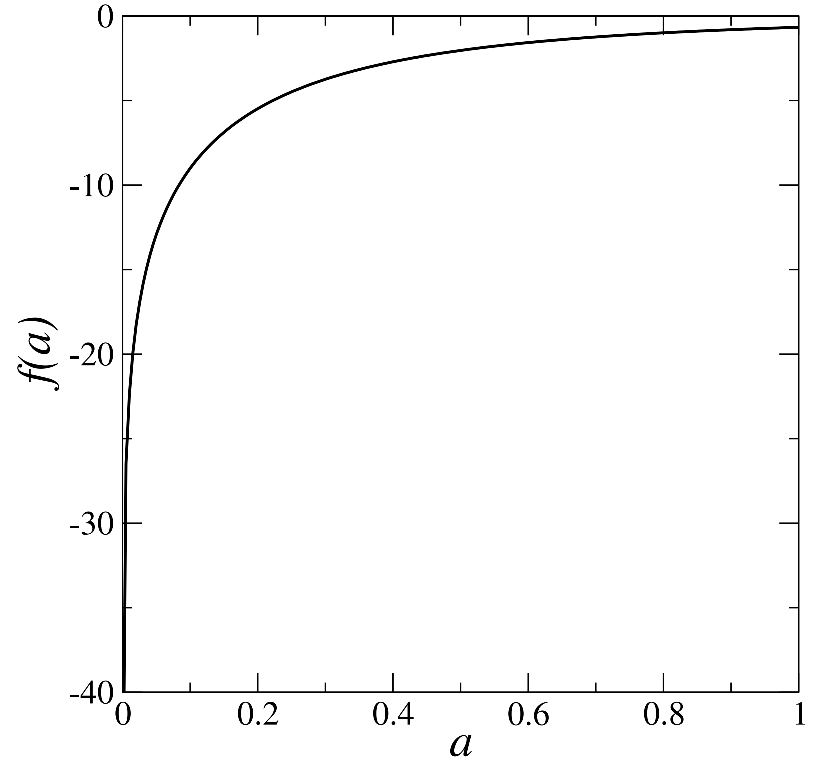


FIG. 1: Plot of function $f$ vs $a$ for $0 < a < 1$. $f(a)$ is negative over the entire range of $a$.

and $\phi'_a$ is the derivative of $\phi_a$. The integral in Eq. (28) can be computed analytically, leading to

$$f(a) = \frac{2}{3} \frac{\sqrt{1-a^2}\left(a^2+14\right) + \left(6a^2+9\right) \log\left(\frac{a}{\sqrt{1-a^2}+1}\right)}{\left(1-a^2\right)^{5/2}} \tag{29}$$

Since $c, b$ are positive, one needs to examine the function $f(a)$ in the interval $0 < a < 1$. One obtains that $f(a)$, and, correspondingly, $d$, are always negative for all values of $a$, see Fig. 1. Therefore, the band solution is always unstable with respect to long-wavelength transverse undulations. However, the solution can be stabilized in a relatively small system of size $L_x$ in the $x$-direction if $L_x$ becomes small compared to the most unstable wavelength. Function $f(a)$ can be also evaluated analytically in two limiting cases:

$$f(a) = 6 \log \frac{a}{2} + \frac{28}{3} + O(a^2) < 0 \text{ for } a \to 0 \tag{30}$$

$$f(a) = -\frac{2}{3} - \frac{44(1-a)}{35} + O\left((1-a)^{3/2}\right) < 0 \text{ for } a \to 1 \tag{31}$$
